# Supplementary material for: A Multiobjective Approach for Sector Duration Optimization in Stereotactic Radiosurgery Treatment Planning
Source: arXiv:2104.13878 source file (2022-05-21)
Supplement: Supplementary file 1 [file appendix_proofs.tex]

\section{Proofs}
\label{app:proofs}

% In this section, 
We provide proofs for the propositions presented in the paper.
%, as well as their statements for the sake of completeness. 
We number the equations in this section with a prefix of “OS”.

\subsection{Proof of Proposition \ref{prop:efficiency}}\label{app:efficiency_proof}
{\it \input{Propositions/prop_eps_cons_correctness}}
\input{Propositions/proof_eps_cons_correctness}

\subsection{Proof of Proposition \ref{prop:underdose_UB}}
{\it \input{Propositions/prop_underdose_UB_appendix}}
\input{Propositions/proof_underdose_UB}

\subsection{Proof of Proposition \ref{prop:BOT_LB}}
{\it \input{Propositions/prop_BOT_LB_appendix}}
\input{Propositions/proof_BOT_LB}

\subsection{Proof of Proposition \ref{prop:equiv1}}
{\it \input{Propositions/prop_repeating_sols_1}}
\input{Propositions/proof_repeating_sols_1}
